# Supplementary material for: Selective Forgetting: Advancing Machine Unlearning Techniques and Evaluation in Language Models
Source: arXiv:2402.05813 source file (2024-12-16)
Supplement: Supplementary file 1 [file appendix.tex]

% \newpage
\appendix

\section{Full Experimental Results}
\label{sec:app:full_results}
\begin{table*}[t]
    \setlength{\tabcolsep}{1.1mm}\small
    \newcommand{\tabincell}[2]{\begin{tabular}{@{}#1@{}}#2\end{tabular}}
    \begin{center}
        \resizebox{\linewidth}{!}{
            \begin{tabular}{ll|cccc|c|cc|ccccc|c}
                \toprule
                \multirow{2}{*}{Models} & & \multicolumn{4}{c}{\tabincell{c}{Forget Evaluation}} & \multicolumn{9}{c}{\tabincell{c}{Classification Test Set Evaluation}} \\
                \cmidrule(lr){3-6}\cmidrule(lr){7-14}\cmidrule(lr){15-15}
                & & EL & MA & S-EL & S-MA & Hella. & Wino. & COPA  & ARC-E & ARC-C & Piqa  & MathQ & PubQ & Avg. \\
                \midrule
                \rowcolor[rgb]{0.93,0.93,0.93}
                \multirow{4}{*}{\tabincell{l}{GPT-Neo \\ 125M}} & Original &31.5 &76.9 &22.0 &62.4  &28.2 &51.5 &60.2 &46.1 &20.3 &63.4 &22.5 &57.2  &43.7 \\
                & \textsc{Kul} &0.2 &26.8 & 1.3 &22.9  &27.1 &52.5 &50.8 &38.5 &19.1 &60.1 &22.1 &57.2  & 40.9\\
                & \shortname &1.0 &29.5 &0.3 &16.1  &27.5 &49.3 &55.5 &37.9 &25.0 &58.9 &20.8  &52.8 &41.0  \\
                \midrule
                \rowcolor[rgb]{0.93,0.93,0.93}
                \multirow{4}{*}{\tabincell{l}{GPT-Neo \\ 1.3B}} & Original &60.4 &91.1 &44.6 &81.6  &37.0 &54.5 &69.2 &56.6 &25.8 &70.3 &21.9 &53.4  &48.6 \\
                & \textsc{Kul} &0.3 &27.2 &1.4 &23.9  &36.7 &55.6 &69.2 &54.0 &25.4 &70.1 &21.6 &52.8  &48.2 \\
                % & $\Delta$(\textsc{Kul},Ori) &- &- &- &-  &($\downarrow0.6$) &($\uparrow0.3$) &($\downarrow0.6$) &($\downarrow2.9$) &($\uparrow0.4$) &($\downarrow1.0$) &(0.0) &($\downarrow1.0$)  &($\downarrow0.6$) \\
                & \shortname &0.6 &29.4 &1.9 &23.6  &36.6 &55.0 &69.3 &54.6 &25.8 &69.5 &21.8  &51.4 & 48.0\\
                \midrule
                \rowcolor[rgb]{0.93,0.93,0.93}
                \multirow{4}{*}{\tabincell{l}{GPT-Neo \\ 2.7B}} & Original &66.6 &93.1 &49.5 &82.5  &40.7 &55.9 &74.2 &59.6 &24.6 &72.9 &21.4 &56.6  &50.7 \\
                & \textsc{Kul} &0.5 &29.8 &1.7 &23.0  &40.8 &55.8 &67.3 &54.5 &29.8 &72.8 &21.5 & 56.9  &49.9 \\
                & \shortname &0.3 &18.6 &1.0 &14.6  &40.3 &55.4 & 70.5 &56.2 &27.2 &73.0 &22.0 & 56.7   &50.2 \\
                \bottomrule
            \end{tabular}
        }
    \end{center}
    % \vskip -1em
    \caption{\label{tab:main_results_classification} Full comparison results (in \%) on forget set ($d$=32) and 8 classification datasets. }
    % \vskip -1em
\end{table*}

\begin{table*}[t]
\setlength{\tabcolsep}{1.1mm}\small
\newcommand{\tabincell}[2]{\begin{tabular}{@{}#1@{}}#2\end{tabular}}
\begin{center}
\resizebox{0.65\linewidth}{!}{
\begin{tabular}{ll|cc|cc|cc|cc|cc}
\toprule
\multirow{2}{*}{Models} & & \multicolumn{10}{c}{ \tabincell{c}{Dialogue Test Set Evaluation}}
\\
\cmidrule(lr){3-12}
&& \multicolumn{2}{c}{ \tabincell{c}{WoW}} & \multicolumn{2}{c}{ \tabincell{c}{ED}} & \multicolumn{2}{c}{ \tabincell{c}{BST}}  & \multicolumn{2}{c}{ \tabincell{c}{WoI}} &  \multicolumn{2}{c}{ \tabincell{c}{Avg.}}\\
\cmidrule(lr){3-4}\cmidrule(lr){5-6}\cmidrule(lr){7-8}\cmidrule(lr){9-10}\cmidrule(lr){11-12}
& &F1 & PPL &F1 & PPL &F1 & PPL &F1 & PPL &F1 & PPL \\
\midrule
\rowcolor[rgb]{0.93,0.93,0.93}
                \multirow{5}{*}{\tabincell{l}{GPT-Neo \\ 125M}} & Original  &10.5 &45.5 &8.4 &41.1 &9.6 &44.9 &11.2 &42.8  &7.4 &43.6 \\
\midrule
& \textsc{Kul}   &1.3 &654.4 &1.2 &438.1 &0.7 &526.1 &1.1 &537.8  &1.1 &539.1 \\
% & \;\;$\Delta$(\textsc{Kul},Ori)  &($\downarrow$5.9) & &($\downarrow$5.5) & &($\downarrow$7.5) & &($\downarrow$8.4) &  &($\downarrow$6.8) & \\
& \shortname  &8.1 &214.9 &7.0 &152.8 &7.2 &185.0 &8.7 &166.6  &7.8 &179.8 \\

% & \;\;$\Delta$(\shortname,Ori) & & & & & & & &  & & \\
\midrule
\rowcolor[rgb]{0.93,0.93,0.93}
                \multirow{5}{*}{\tabincell{l}{GPT-Neo \\ 1.3B}} &Original  &12.7 &26.5 &10.5 &25.3 &12.1 &27.0 &13.8 &25.0  &12.3 &26.0 \\
\midrule
& \textsc{Kul} &11.2 &33.0 &9.3 &31.9 &9.9 &33.6 &11.2 &31.1 &10.4 &32.4 \\
% & \;\;$\Delta$(\textsc{Kul},Ori) & & & & & & & &  & & \\
& \shortname  &12.3 &28.9 &10.2 &27.9 &10.7 &29.4 &12.3 &27.0  &11.4 &28.3 \\
% & \;\;$\Delta$(\shortname,Ori) & & & & & & & &  & & \\
\midrule
\rowcolor[rgb]{0.93,0.93,0.93}
                \multirow{5}{*}{\tabincell{l}{GPT-Neo \\ 2.7B}} &Original  &12.3 &23.5 &10.8 &22.9 &12.5 &24.0 &13.5 &22.6  &12.3 &23.3 \\
\midrule
& \textsc{Kul} &10.8 &30.8 &8.8 &29.7 &9.7 &30.9 &10.9 &29.0  &10.1 &30.1 \\
% & \;\;$\Delta$(\textsc{Kul},Ori) & & & & & & & &  & & \\
& \shortname  &11.3 &27.0 &9.2 &26.6 &11.0 &27.3 &12.0 &26.0  &10.9 &26.7 \\
% & \;\;$\Delta$(\shortname,Ori) & & & & & & & &  & & \\

\bottomrule
\end{tabular}
}
\end{center}
% \vskip -1em
\caption{\label{tab:main_results_dialogue} 
Full comparison results (in \%) with $d$=32 setting on 4 dialogue datasets.  
}
% \vskip -1em
\end{table*}
\begin{table}[t]
    \setlength{\tabcolsep}{2.1mm}\small
    \newcommand{\tabincell}[2]{\begin{tabular}{@{}#1@{}}#2\end{tabular}}
    \begin{center}
        \resizebox{\linewidth}{!}{
            \begin{tabular}{l|cc|cc|cc|cc|cc}
                \toprule
                \multirow{2}{*}{Models} & \multicolumn{2}{c}{\tabincell{c}{$n$=1}} & \multicolumn{2}{c}{\tabincell{c}{$n$=4}} & \multicolumn{2}{c}{\tabincell{c}{$n$=8}} & \multicolumn{2}{c}{\tabincell{c}{$n$=10}} & \multicolumn{2}{c}{\tabincell{c}{$n$=15}} \\
                \cmidrule(lr){2-3}\cmidrule(lr){4-5}\cmidrule(lr){6-7}\cmidrule(lr){8-9}\cmidrule(lr){10-11}
                &EL & S-EL &EL & S-EL &EL & S-EL &EL & S-EL &EL & S-EL \\
                \midrule
                125M  &43.4 &7.71 &2.89 &0.56 &1.13 &0.36 &1.02 &0.33 &0.44 &0.35   \\
                1.3B  &61.0 &11.9 &2.69 &2.2 &0.82 &1.94 &0.59 &1.89 &0.27 &1.95   \\
                2.7B  &79.8 &4.49 &0.70 &0.88 &0.28 &0.92 &0.26 &0.95 &0.19 &1.06   \\
                \bottomrule
            \end{tabular}
        }
    \end{center}
    % \vskip -1em
    \caption{\label{tab:el_n} Results of EL$_n$ and S-EL$_n$ with varying $n$.}
    % \vskip -1em
\end{table}

The results reported in the main paper are average scores across multiple classification and dialogue systems. Here we further present the scores on each dataset in \Cref{tab:main_results_classification} and \Cref{tab:main_results_dialogue}. \Cref{tab:main_results_classification} provides an overview of the performance on forget set and classification datasets, while Table \Cref{tab:main_results_dialogue} reports the performance on dialogue datasets. 

\section{Experimental/Annotation Details}\label{sec:appendix_details}
\paragraph{Backward Verification of Annotated Spans.} 
In Section~\ref{ssec:model:forgetting_span}, we discussed the two-stage offline sensitive annotation method. Here, we provide additional details about the backward verification. We prompt  \texttt{gpt-3.5-turbo-0613} with the following instruction:
\begin{quote}
\vspace{-0.5\baselineskip} 
\begin{adjustwidth}{-0.4cm}{-0.4cm}
\definecolor{Lightgray}{RGB}{130,130,130}
\textit{
Given the text span shown below: \\
\colorbox{Lightgray}{\color{white}{\textit{Sensitive Span}}} \\
Please rate it on a scale from \{0, 1, 2\}. Assign 0 for non-sensitive, 2 for sensitive, and 1 for somewhat sensitive. Sensitivity is defined here as information that could potentially help identify details about a specific organization, event, person, or other entities. Please first analyze the text content and then output a new single line containing only the integer rating.
}
\end{adjustwidth}
\vspace{-0.5\baselineskip} 
\end{quote}
Based on the returned ratings, we filter out the sensitive spans labeled with 0.

\paragraph{NER-based Annotation.} We perform Named Entity Recognition (NER) based annotation using spaCy\footnote{\url{https://spacy.io/}} and the \texttt{en\_core\_web\_sm} model on English text.

\paragraph{Human Annotation of Sensitive Span.} 
Two annotators were invited to independently annotate the same set of 50 randomly sampled instances for the presence of sensitive spans. After independent annotation, inner discussions are conducted to achieve agreement on the annotated spans.

\section{Further Analysis}
\paragraph{Efficiency of Proposed Evaluation Metrics.}
The evaluation metrics EL and MA are used as monitors (i.e., forgetting threshold) to determine whether unlearning needs to be stopped. Therefore, the efficiency in calculating these metrics also plays a role in training efficiency. We emphasize that our proposed metrics, S-EL and S-MA, have an additional advantage in terms of computational efficiency. As seen in \Cref{tab:annotation_statistic}, the annotated sensitive proportions are mostly below $10\%$, indicating that compared to EL and MA, S-EL and S-MA can achieve approximately a 10-fold acceleration in computation. This efficiency gain is attributed to their shared computational complexity, which scales similarly with sequence length.
% As evaluation metrics EL and MA are utilized as monitors (forgetting threshold) to decide whether needing an early stop, the efficiency of calculating these metrics also plays a role in unlearning efficiency. We emphasize that our proposed metrics S-EL and S-MA have one additional advantage in calculation efficiency. From \Cref{tab:annotation_statistic}, the annotated sensitive proportions are mostly below $10\%$, indicating that compared to EL and MA, S-EL and S-MA can achieve approximately a 10-fold acceleration in computation, as they share a computational complexity that scales similarly with sequence length.

\paragraph{Varying $n$ in the Calculation of S-EL$_{n}$.}
In our main experiments, we mainly report results of S-EL$_{10}$. Here we showcase the outcomes with varying $n$ values for the S-EL metric, alongside EL, in order to assess its impact. As illustrated in \Cref{tab:el_n}, it is evident that S-EL demonstrates a tendency to remain smooth when $n \ge 4$, whereas EL consistently shows a decline. This pattern is primarily attributed to the fact that the average length of annotated sensitive spans should be approximately $4$. Furthermore, this observation underscores a notable advantage of our proposed S-EL over EL, as it exhibits greater robustness in the face of variations.
