# Supplementary material for: Selective Forgetting: Advancing Machine Unlearning Techniques and Evaluation in Language Models
Source: arXiv:2402.05813 source file (2024-12-16)
Supplement: Supplementary file 2 [file appendix_el_n.tex]

\begin{table}[t]
    \setlength{\tabcolsep}{2.1mm}\small
    \newcommand{\tabincell}[2]{\begin{tabular}{@{}#1@{}}#2\end{tabular}}
    \begin{center}
        \resizebox{\linewidth}{!}{
            \begin{tabular}{l|cc|cc|cc|cc|cc}
                \toprule
                \multirow{2}{*}{Models} & \multicolumn{2}{c}{\tabincell{c}{$n$=1}} & \multicolumn{2}{c}{\tabincell{c}{$n$=4}} & \multicolumn{2}{c}{\tabincell{c}{$n$=8}} & \multicolumn{2}{c}{\tabincell{c}{$n$=10}} & \multicolumn{2}{c}{\tabincell{c}{$n$=15}} \\
                \cmidrule(lr){2-3}\cmidrule(lr){4-5}\cmidrule(lr){6-7}\cmidrule(lr){8-9}\cmidrule(lr){10-11}
                &EL & S-EL &EL & S-EL &EL & S-EL &EL & S-EL &EL & S-EL \\
                \midrule
                125M  &43.4 &7.71 &2.89 &0.56 &1.13 &0.36 &1.02 &0.33 &0.44 &0.35   \\
                1.3B  &61.0 &11.9 &2.69 &2.2 &0.82 &1.94 &0.59 &1.89 &0.27 &1.95   \\
                2.7B  &79.8 &4.49 &0.70 &0.88 &0.28 &0.92 &0.26 &0.95 &0.19 &1.06   \\
                \bottomrule
            \end{tabular}
        }
    \end{center}
    % \vskip -1em
    \caption{\label{tab:el_n} Results of EL$_n$ and S-EL$_n$ with varying $n$.}
    % \vskip -1em
\end{table}
